# Supplementary material for: Temporal scaling in information propagation
Source: arXiv:1311.4336 source file (2014-06-18)
Supplement: Supplementary file 1 [file influ-infer-SI.pdf]

# Supplementary Materials: Temporal scaling in information propagations

Junming Huang[1] Chao Li[1,2] Wen-Qiang Wang[2]
Hua-Wei Shen[1] Guojie Li[1] Xue-Qi Cheng[1]

1 Institute of Computing Technology, Chinese Academy of Sciences, Beijing, People's Republic of China
2 Web Sciences Center, School of Computer Science and Engineering, University of Electronic Science and Technology of China, Chengdu, Sichuan, People's Republic of China
∗ Corresponding Author: shenhuawei@ict.ac.cn

## Contents

**S1 Dataset** **1**

**S2 Problem statement** **3**

**S3 Inference** **3**

**S4 Baselines** **5**

**S5 Evaluation metrics** **6**

**S6 Experiment settings** **7**

## S1 Dataset

The dataset we use in all experiments is a benchmark dataset that was released as a task of the 13th International Conference on Web Information System Engineering (WISE 2012 Challenge). The dataset contains crawled users and retweeting behaviors between Aug 24, 2009 and Dec 31, 2011 [1] from a Chinese social media website Sina Weibo (http://www.weibo.com). We cleaned the data by removing inactive users and unpopular messages. We also removed spam users who abnormally retweet a single message for hundreds of times. We built a directed edge $(v_i, v_j)$ if the user $v_j$ directly retweeted no less than 10 messages

[1] WISE officially declares the end date of crawling as Dec 2011. However, we actually find records in Jan and Feb 2012.

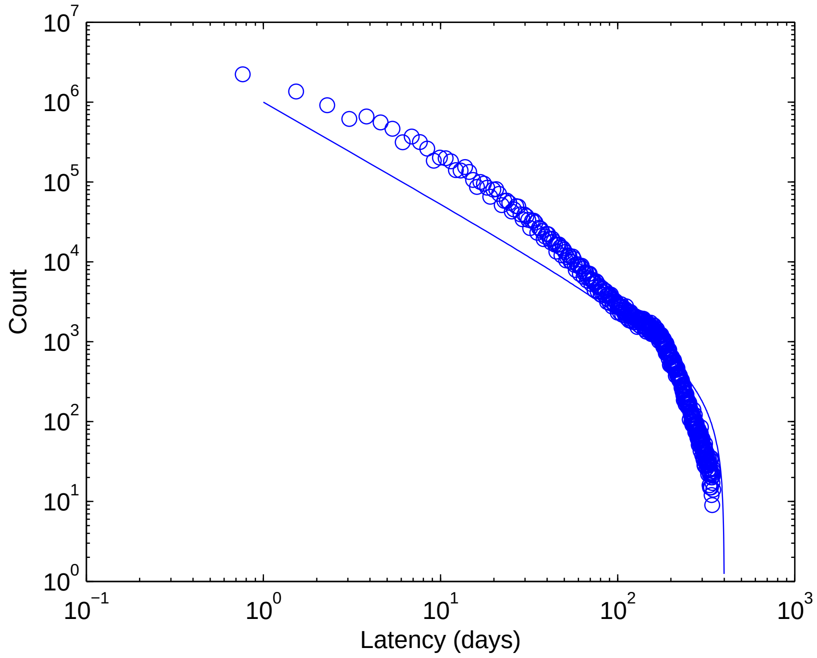


Figure S1: Distribution of latency on all data. The fast decaying tail attributes to incomplete crawling, as fitted with a solid curve representing the modification of such an incomplete crawling.

that were previously posted or retweeted by $v_i$. We remove cascades whose propagation trees are not completed crawled, i.e., some retweeting behaviors are missing. Basic statistics of the dataset is reported in Table S1.

The distribution of latency in the dataset is shown in Figure S1, with a tail decaying faster than a power law. That tail does not mean that the power-law decaying manner is violated, but instead attributes to the incomplete crawling. Suppose the crawling time window lasts for $L$ days. An example with $t_{k,i}$ located in the crawling time window, is observed with $l$-day latency only if the time stamp $t_{k',j} = t_{k,i} - \tau_{i,j,k}$ is also located within the crawling window. Suppose $t_{k,i}$ is uniformly distributed in the crawling window, such an example is observed with the probability $\frac{L-l}{L}$. Specifically, instead of the formula $P(\tau) \propto \tau^{-1.27}$ suggested in Figure 1(e), a slight modification $P(\tau) \propto \tau^{-1.27} * \frac{400-\tau}{400}$ fits the observed data well, shown as a solid curve in Figure S1. The length is set to 400 days for best fit, much shorter than the total length of the dataset crawling window (Aug 2009 - Dec 2011), implying that most crawled records concentrate in the last year as the rapid growing of Sina Weibo. Therefore, in the report we do not show the tail with incomplete data.

## S2 Problem statement

Consider an underlying social network (graph) $G = (V, E)$. A node $v_i \in V$ is an individual. An edge $(v_i, v_j) \in E$ means that $v_j$ follows $v_i$, i.e., a message could propagate from $v_i$ to $v_j$. We say $v_i$ is a *followee* of $v_j$, and $v_j$ a *follower* of $v_i$.

In a social media scenario, we define a cascade as a tree consisting of an *original message* and all messages retweeted from it. With the typical setting of Independent Cascade model, in a cascade each node can be in either state: active or inactive. Once an individual retweets a message in the cascade, she turns into the active state and is added into the cascade. Otherwise she remains inactive. Every time $v_i$ posts or retweets a message, she attempts to activate all her inactive followers with one chance. An inactive follower $v_j$ chooses either to become active by retweeting *that* message posted/retweeted by $v_i$, or to stay inactive by neglecting the attempt. If $v_j$ retweets it, we say $v_i$ successfully activates $v_j$ and record the example $\{v_i, v_j, k\}$ as a *positive example*, denoted as $\delta_{i,j,k} = 1$. If $v_j$ neglects it, we say $v_i$ fails to activate $v_j$ and record the example $\{v_i, v_j, k\}$ as a *negative example*, denoted as $\delta_{i,j,k} = 0$.

For each example $\{v_i, v_j, k\}$, its latency $\tau_{i,j,k}$ is recorded to measure the time span since the latest time $v_j$ retweets a message from $v_i$ till the time $v_j$ decides to retweet the message $k$ from $v_i$ or not. For a positive example, the decision time equals to $t_{k,j}$, the time $v_j$ retweets message $k$ posted/retweeted by $v_i$. For a negative example, the decision time equals to $t_{k,j}$, the time $v_i$ posts/retweets the message $k$ and attempts to activate $v_j$. The latter is an approximation since we do not know the exact time when $v_j$ decides not to retweet, however, the error (indeed the latency) is negligible since a latency is usually several minutes or hours [S2] while a typical latency lasts for several days or weeks.

In an information cascade $C_k$, all positive examples consist a directed tree with a sequence of events tracking how information $k$ propagates on $G$.

$$C_k = \{(v_i, v_j, t_{k,j}), (v_j, v_j', t_{k,j'}), \dots\}$$

where each tuple $(v_i, v_j, t_{k,j})$ describes an event that a node $v_i$ activates its follower node $v_j$ at time $t_{k,j}$. If a node is not activated with message $k$, it does not appear in the sequence $C_k$.

## S3 Inference

For *Deday model*, hidden variables $\{\boldsymbol{q}, \boldsymbol{\alpha}\}$ are inferred with a maximum a posteriori probability strategy. Priors are introduced to avoid over-fitting, since a typical edge carries few examples that could be insufficient to support a stable statistical estimator. For the Decay model, we assign two priors to the two classes of hidden variables respectively, i.e., $q_{i,j}$ follows an exponential distribution $Exp(\lambda)$ bounded in $[0, 1]$, while $\alpha_{i,j}$ follows a log-normal distribution $\ln N(\mu, \sigma^2)$, capturing the prior knowledge learned in the empirical study that $\alpha$ is roughly 1.0 (slope in Figure 1(f)) and $\ln q$ is close to 0.1 (intersect in Figure 1(f)).

$$P(q_{i,j}) = \frac{\lambda}{1-e^{-\lambda}} e^{-\lambda q_{i,j}}, \lambda > 0 \tag{S1}$$

$$P(\alpha_{i,j}) = \frac{1}{\alpha_{i,j}\sqrt{2\pi\sigma^2}} e^{-\frac{(\ln \alpha_{i,j}-\mu)^2}{2\sigma^2}}, \mu \in R, \sigma > 0$$

Then the posterior distribution of hidden parameters should be

$$P(\boldsymbol{q}, \boldsymbol{\alpha}|data) \propto \prod_{(v_i,v_j)\in E} \frac{\lambda}{1-e^{-\lambda}} e^{-\lambda q_{i,j}} \frac{1}{\alpha_{i,j}\sqrt{2\pi\sigma^2}} e^{-\frac{(\ln \alpha_{i,j}-\mu)^2}{2\sigma^2}} \prod_{k\in K^+_{i,j}} q_{i,j}\tau_{i,j,k}^{-\alpha_{i,j}} \prod_{k\in K^-_{i,j}} \left(1 - q_{i,j}\tau_{i,j,k}^{-\alpha_{i,j}}\right),$$

where $K^+_{i,j}$ is the set of messages that $v_i$ posts/retweets and then $v_j$ retweets, while $K^-_{i,j}$ is the set of messages that $v_i$ posts/retweets and then $v_j$ ignores.

Maximizing the above posterior probability against hidden parameters, we obtain a maximum a posteriori probability estimation. Practically we use the logarithm of the above posterior probability instead for ease of float calculations.

$$\begin{aligned}\{\hat{q}, \hat{\alpha}\} &= \operatorname*{argmax}_{q,\alpha} \ln P(\boldsymbol{q}, \boldsymbol{\alpha}|data) \\ &= \operatorname*{argmax}_{q,\alpha} \sum_{(v_i,v_j)\in E} \Bigg( \ln\lambda - \ln(1-e^{-\lambda}) - \lambda q_{i,j} - \frac{1}{2}\ln(2\pi\sigma^2) - \ln\alpha_{i,j} - \frac{1}{2\sigma^2}(\ln\alpha_{i,j}-\mu)^2 \\ &+ \sum_{k\in K^+_{i,j}} (\ln q_{i,j} - \alpha_{i,j}\ln\tau_{i,j,k}) + \sum_{k\in K^-_{i,j}} \ln\left(1 - q_{i,j}\tau_{i,j,k}^{-\alpha_{i,j}}\right)\Bigg).\end{aligned} \tag{S2}$$

In practice we choose simple values of hyperparameters $\lambda = 1$, $\mu = 0$ and $\sigma = 1$, start from a random initial guess and iteratively update parameter values with partial gradients of the logarithm posterior probability as follows, until convergence.

$$\frac{\partial}{\partial q_{i,j}} \ln P(\boldsymbol{q}, \boldsymbol{\alpha}|data) = -\lambda + \sum_{k\in K^+_{i,j}} \frac{1}{q_{i,j}} - \sum_{k\in K^-_{i,j}} \frac{1}{\tau_{i,j,k}^{\alpha_{i,j}} - q_{i,j}} \tag{S3}$$

$$\begin{aligned}&\frac{\partial}{\partial \alpha_{i,j}} \ln P(\boldsymbol{q}, \boldsymbol{\alpha}|data) \\ &= -\frac{1 + (\ln\alpha_{i,j} - \mu)/\sigma^2}{\alpha_{i,j}} - \sum_{k\in K^+_{i,j}} \ln(\tau_{i,j,k}) - \sum_{k\in K^-_{i,j}} \frac{q_{i,j}\ln(\tau_{i,j,k})}{q_{i,j} - \tau_{i,j,k}^{\alpha}}\end{aligned} \tag{S4}$$

In order to validate the consistence of our models, we create a synthetic dataset to examine whether our inference process can correctly recover hidden parameters $\{\boldsymbol{q}, \boldsymbol{\alpha}\}$ if user behaviors are indeed generated with our probability models. We build a single directed edge $(Alice, Bob)$ with a random selected $q_{Alice,Bob} \in [0,1]$ and $\alpha_{Alice,Bob} \in [0,2]$ for example. At every time step $t_k$, *Alice* posts a message $k$, and *Bob* immediately decides whether to retweet $k$ with a probability described in Equ. 2, where the latency $\tau_{Alice,Bob,k}$ is calculated by $t_k$ minus the latest time *Bob* retweeted a message. The probability of the first message is set to 1 in order to avoid the difficulty in calculating latency with no previous retweeting behaviors. We record a positive example if *Bob* decides to retweet, while a negative example if *Bob* neglects. After *Bob* retweets a predefined number of messages, e.g., 10 messages, we stop the simulation and use the generated examples to train our model to estimate $q_{Alice,Bob}$ and $\alpha_{Alice,Bob}$. We vary the predefined number of retweeted messages in simulations from 10 to 100, and build $10,000$ edges to repeat the simulations. The accuracy of estimation $\{\tilde{\boldsymbol{q}}, \tilde{\boldsymbol{\alpha}}\}$ is measured with *mean absolute error*, i.e., $E\left[|\tilde{q} - q|\right]$ and $E\left[|\tilde{\alpha} - \alpha|\right]$. As reported in Figure S2, our models accurately recover the hidden parameters with an MAE near 0.2 requiring only 10 retweets, and the estimation error further decreases to a fair level when the number of retweeting behaviors grows.

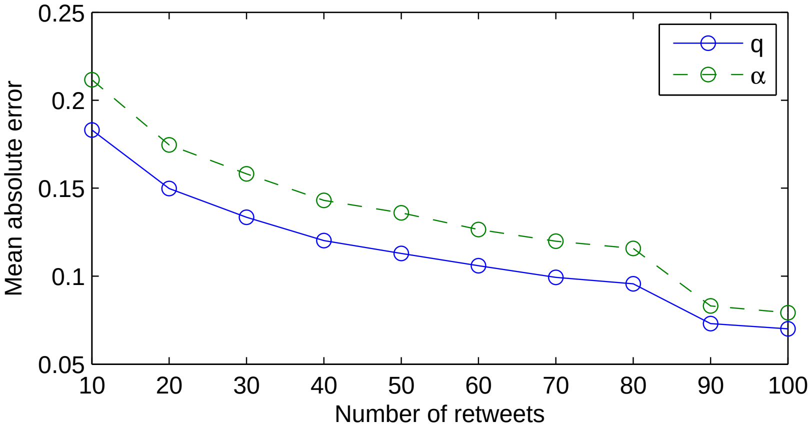


Figure S2: Estimating hidden parameters on synthetic data. The mean absolute error between the estimation and the ground truth decreases with increasing number of retweeting behaviors.

## S4 Baselines

Following 4 mainstream baselines are implemented to compare with our models. Those baselines are proposed to estimate propagation probabilities based on

retweeting behavior logs only. Other methods requiring user profile or message content are not applicable in the dataset.

- **MLE**. The simplest algorithm outputs an edge propagation probability as the ratio of successful attempts over all attempts on that edge. The method provides a maximum-likelihood estimation, assuming static probabilities.
- **Static Bernoulli** and **Static PC Bernoulli** proposed in [S3]. The method scans action log containing the activation time stamps of each node in each cascade, on a known social network. We implement all 12 versions described in [S3] and for simplicity only report the two with the best performance on the dataset, namely **Static Bernoulli** with static Bernoulli propagation probabilities and **Static PC Bernoulli** with a partial credit strategy.
- **EM** algorithm proposed in [S4]. On a known social network, the method assumes a static propagation probability on each edge and runs a maximum-likelihood estimation on the action log containing only activation time stamps of each node in each cascade. It considers discrete time rather than real continuous time, i.e., if $v_i$ activates $v_j$ in a cascade, their time stamps differ by one. Therefore we slightly modify our dataset to make it appropriate for the method. In each cascade $C_k$, we assign $t_{i,k} = 0$ if node $v_i$ is the root of the cascade, or assign $t_{j,k}$ to the depth of $v_j$ in the cascade from the root node. i.e., we build a directed tree for $C_k$ where each directed edge $(v_i, v_j)$ represents an event that $v_i$ activates $v_j$ in the cascade, and label $t_{i,k}$ as the depth of $v_i$ in the tree.

**NetInf** [S5] was also implemented. That method simultaneously estimates an unknown social network and propagation probabilities given action log. It leverages the waiting time of each retweeting behavior to estimate propagation probabilities. However, it meets a serious scalability problem that it cannot finish inference on a real-world scale large dataset such as what we use in this paper within acceptable time. Tests on a smaller sample shows that its performance is no better than **EM**. Therefore we didn't report its performance in our report.

# S5 Evaluation metrics

*Perplexity*: the metric used to measure the ability a probabilistic model (e.g., our Decay model) generates observed examples. In our paper, we train a probabilistic model on the training set and evaluate it with its perplexity on the testing set, in order to measure how the testing examples surprise the trained model. A lower perplexity indicates better performance.

$$perplexity = e^{-\frac{\sum_{\{v_i, v_j, k\} \in D_{test}} \delta_{i,j,k} \ln \tilde{P}(\delta_{i,j,k}=1) + (1-\delta_{i,j,k}) \ln(1-\tilde{P}(\delta_{i,j,k}=1))}{|D_{test}|}} \tag{S5}$$

where $D_{test}$ represents the testing set, and $\tilde{P}(\delta_{i,j,k} = 1)$ is the estimated probability that $v_j$ retweets message $k$ from $v_i$.

*AUC*: the area under the Receiver Operating Characteristic curve, used to evaluate a binary classification problem, namely retweeting prediction in our experiments. Dislike the perplexity, AUC is independent from the ratio of positive and negative examples, and therefore suitable for datasets where positive and negative examples are imbalanced. AUC is equivalent to the probability that a trained model correctly tells a randomly selected positive example from another randomly selected negative example. Obviously a higher AUC indicates a better model [S1].

# S6 Experiment settings

In the viral marketing experiment, we split the data into 4 groups with respect to example time stamps. Each group contains examples in 30 weeks, divided into a 205-day training phase and a 5-day evaluation phase, as shown in Table S3. In each evaluation phase, we build a propagation network $G' = (V, E')$ as a subgraph of the social network, with edges on which at least one actual retweeting behavior occur in the evaluation phase. Roughly speaking, 1% edges should survive in such a subgraph, since the positive examples occupies about 1% of all examples in the dataset, which reveals that the global average propagation probability is around 0.01. The length of the evaluation phase is then determined such that $|E'| = 0.01|E|$.

# References


[S1] Tom Fawcett. An introduction to roc analysis. *Pattern recognition letters*, 27(8):861–874, 2006.

[S2] Peng Bao, Hua-Wei Shen, Junming Huang, and Xue-Qi Cheng. Popularity prediction in microblogging network: a case study on sina weibo. In *Proceedings of the 22nd international conference on World Wide Web companion*. International World Wide Web Conferences Steering Committee, 2013.

[S3] Amit Goyal, Francesco Bonchi, and Laks V.S. Lakshmanan. Learning influence probabilities in social networks. In *Proceedings of the third ACM international conference on Web search and data mining*, pages 241–250, 1718518, 2010. ACM.

[S4] Kazumi Saito, Ryohei Nakano, and Masahiro Kimura. *Prediction of Information Diffusion Probabilities for Independent Cascade Model*, volume 5179 of *Lecture Notes in Computer Science*, chapter 9, pages 67–75. Springer Berlin Heidelberg, 2008.

[S5] Manuel Gomez-Rodriguez, Jure Leskovec, and Andreas Krause. Inferring networks of diffusion and influence. In *Proceedings of the 16th ACM SIGKDD international conference on Knowledge discovery and data mining*, pages 1019–1028, 1835933, 2010. ACM.

Table S1: Data statistics.

| Statistics | Value |
|---|---|
| Num of users | 496,929 |
| Num of edges | 1,215,116 |
| Num of cascades | 8,005,507 |
| Num of positive (retweeting) examples | 19,688,837 |
| Num of negative (neglecting) examples | 2,126,313,325 |

Table S2: Notations

| Notation | Meaning |
|---|---|
| $v_i \in V$ | Node (user); |
| $(v_i, v_j) \in E$ | Edge where user $v_j$ follows $v_i$; |
| $q_{i,j} \in [0, 1]$ | Base probability associated with the edge $(i, j)$; |
| $\alpha_{i,j} \in (0, +\infty)$ | Decaying parameter associated with the edge $(i, j)$; |
| $t_{k,j}$ | Time stamp when $v_k$ retweets a message $k$; |
| $\delta_{i,j,k}$ | Label to indicate whether a node $v_i$ activates a follower node $v_j$ at time $t_{k,j}$ with a message $k$; |
| $\tau_{i,j,k} \geq 1$ | Latency between the latest time $v_j$ was activated by $v_i$ and the current time $v_j$ was activated by $v_i$ with a message $k$, i.e., $\tau_{i,j,k} = t_{k,i} - t_{k',j}$, where $k'$ is the latest message with which $v_i$ activates $v_j$; |
| $\lambda, \mu, \sigma^2$ | Hyperparameters to provide priors of $\boldsymbol{q}$ and $\boldsymbol{\alpha}$. |

Table S3: Phases in viral marketing experiment.

| Training phase starts | Training phase ends | Evaluation phase starts | Evaluation phase ends |
|---|---|---|---|
| 23 Aug 2009 16:00:00 UTC | 16 Mar 2010 09:59:59 UTC | 16 Mar 2010 10:00:00 UTC | 21 Mar 2010 10:00:00 UTC |
| 26 Mar 2010 10:00:01 UTC | 17 Oct 2010 03:59:59 UTC | 17 Oct 2010 04:00:00 UTC | 22 Oct 2010 04:00:00 UTC |
| 27 Oct 2010 04:00:01 UTC | 19 May 2011 21:59:59 UTC | 19 May 2011 22:00:00 UTC | 24 May 2011 22:00:00 UTC |
| 29 May 2011 22:00:01 UTC | 20 Dec 2011 15:59:59 UTC | 20 Dec 2011 16:00:00 UTC | 25 Dec 2011 16:00:00 UTC |
